# Supplementary material for: USP-Gaussian: Unifying Spike-based Image Reconstruction, Pose Correction and Gaussian Splatting
Source: arXiv:2411.10504 source file (2025-06-25)
Supplement: Supplementary file 1 [file X_suppl.tex]

\clearpage
\setcounter{page}{1}
% \maketitlesupplementary
% {
%    \newpage
%        \twocolumn[
%         \centering
%         \Large
%         \textbf{\thetitle}\\
%         \vspace{0.5em}Supplementary Material \\
%         \vspace{1.0em}
%        ] %< twocolumn
%    }
\onecolumn
{\centering
\Large
\textbf{\thetitle}\\
\vspace{0.5em}Supplementary Material\\
\vspace{1.0em}}
\appendix
\section{Introduction}
In this supplementary material, we first analyze the gradient flow of our joint optimization framework in \cref{sec:sup:theory}, followed by a theoretical demonstration that the outputs of 3DGS and Recon-Net are complementary and the joint optimization strategy provides mutual benefits. Next, we present a more detailed comparison between our proposed framework and previous cascading frameworks in \cref{sec:sup:framework}. Further details regarding our implementation and network architecture can be found in \cref{sec:sup:Implementation} and \cref{sec:sup:network}, respectively. Finally, in \cref{sec:sup:exp}, we provide additional quantitative and qualitative experimental results comparing our method with previous approaches from the perspective of the spike-to-image task.
\section{Theory Anaysis} \label{sec:sup:theory}
\subsection{Gradient Flow}

The total loss for our USP-Gaussian is defined in \cref{equ:final_loss}, formulated as follows:
\begin{equation}
\mathcal{L}_{\text{final}} = \mathcal{L}_{\text{rec}}+\mathcal{L}_{\text{gs}}+\mathcal{L}_{\text{joint}}.
\end{equation}

In the following, we analyze the propagation of gradients for the final loss, depicted in \cref{fig:framework}, with respect to Gaussian primitives $\mathbb{G}$, Recon-Net parameters $\theta$, and poses $\mathbb{P}$.

The gradient of the final loss relative to the Gaussian primitives $\mathbb{G}$ is expressed as:
\begin{align}
&\quad \quad \frac{\partial{\mathcal{L}}_{\text{final}}}{\partial{\mathbb{G}}}=\frac{\partial{\mathcal{L}_{\text{gs}}}}{\partial{\mathbb{G}}}+\frac{\partial{\mathcal{L}_{\text{joint}}}}{\partial{\mathbb{G}}} + \cancel{\frac{\partial\mathcal{L}_{\text{rec}}}{\partial\mathbb{G}}},\\
&\left\{
\begin{aligned}
&\frac{\partial{\mathcal{L}_{\text{gs}}}}{\partial{\mathbb{G}}} = \frac{\partial\mathcal{L}_{\text{gs}}}{\partial\mathbf{E}_{\text{gs}}(\mathcal{T})}\cdot \frac{1}{M}\sum_{m=1}^M\frac{\partial\mathbf{E}_{\text{gs}}(\mathcal{T})}{\partial \mathbf{I}_{\text{gs}}(t_m)}\frac{\partial\mathbf{I}_{\text{gs}}(t_m)}{\partial\mathbb{G}}\\
&\frac{\partial{\mathcal{L}_{\text{joint}}}}{\partial{\mathbb{G}}} = 
\frac{1}{M}\sum_{m=1}^M\frac{\partial{\mathcal{L}_{\text{joint}}}}{\partial{\mathbf{I}_{\text{gs}}(t_m)}}\frac{\partial\mathbf{I}_{\text{gs}}(t_m)}{\partial \mathbb{G}} \\
&\frac{\partial{\mathcal{L}_{\text{rec}}}}{\partial{\mathbb{G}}} = 0
\end{aligned}
\right.
\end{align}
where $\mathbf{E}_{\text{gs}}(\mathcal{T})$ denotes the blurry image synthesized by averaging the sequence projected by 3DGS during the interval $\mathcal{T}$.

The gradient of the final loss concerning the pose set $\mathcal{P}$ is formulated as:
\begin{align}
\frac{\partial{\mathcal{L}}_{\text{final}}}{\partial{\mathbb{P}}}&=\frac{\partial{\mathcal{L}_{\text{gs}}}}{\partial{\mathbb{P}}}+\frac{\partial{\mathcal{L}_{\text{joint}}}}{\partial{\mathbb{P}}} + \cancel{\frac{\partial{\mathcal{L}_{\text{rec}}}}{\partial{\mathbb{P}}}}
\\
&=\frac{\partial{\mathcal{L}_{\text{gs}}}}{\partial{\mathbb{G}}}\frac{\partial\mathbb{G}}{\partial\mathbb{P}}+\frac{\partial{\mathcal{L}_{\text{joint}}}}{\partial{\mathbb{G}}}\frac{\partial\mathbb{G}}{\partial\mathbb{P}}.
\end{align}

Further details regarding the calculation of $\frac{\partial\mathbb{G}}{\partial\mathbb{P}}$ can be referred to in BAD-Gaussian.

The gradient of the final loss with respect to the parameters of the Recon-Net is:
\begin{align}
&\quad \quad \quad \quad \quad \quad \quad \quad \quad \quad \frac{\partial{\mathcal{L}}_{\text{final}}}{\partial\theta}=\frac{\partial{\mathcal{L}_{\text{rec}}}}{\partial{\theta}}+\frac{\partial{\mathcal{L}_{\text{joint}}}}{\partial{\theta}} + \cancel{\frac{\partial\mathcal{L}_{\text{gs}}}{\partial\theta}}, \\
&
\left\{
\begin{aligned}
&\frac{\partial{\mathcal{L}_{\text{rec}}}}{\partial{\theta}} = \frac{1}{N}\sum_{n=1}^N\frac{\partial\mathcal{L}_{\text{rec}}}{\partial\mathbb{L}_{\text{rec}}(M_n,\mathcal{T}_n)}\frac{\partial{\mathbb{L}_{\text{rec}}(M_n,\mathcal{T}_n)}}{\partial\mathbf{E}_{\text{rec}}(\mathcal{T}_{n})}\cdot\frac{1}{M_n}\sum_{m=1}^{M_n}\frac{\partial\mathbf{E}_{\text{rec}}(\mathcal{T}_n) }{\partial\mathbf{I}(t_m^n)}\frac{\partial\mathbf{I}(t_m^n)}{\partial\theta} \\
&\frac{\partial{\mathcal{L}_{\text{joint}}}}{\partial{\theta}} = \frac{1}{M}\sum_{m=1}^M\frac{\partial{\mathcal{L}_{\text{joint}}}}{\partial{\mathbf{I}_{\text{rec}}(t_m)}}\frac{\partial\mathbf{I}_{\text{rec}}(t_m)}{\partial \theta} \\
&\frac{\partial{\mathcal{L}_{\text{gs}}}}{\partial{\theta}} = 0
\end{aligned}
\right.
\end{align}
where $\mathbf{E}_{\text{rec}}(\mathcal{T}_n)$ represents the blurry image obtained by averaging the sequence reconstructed by Recon-Net during the sub-interval $\mathcal{T}_{n}$ and $t_m^n$ denotes the timestamp of the $m$-th frame within exposure $\mathcal{T}_{n}$.

\begin{figure}
    \centering
    \includegraphics[width=1\linewidth]{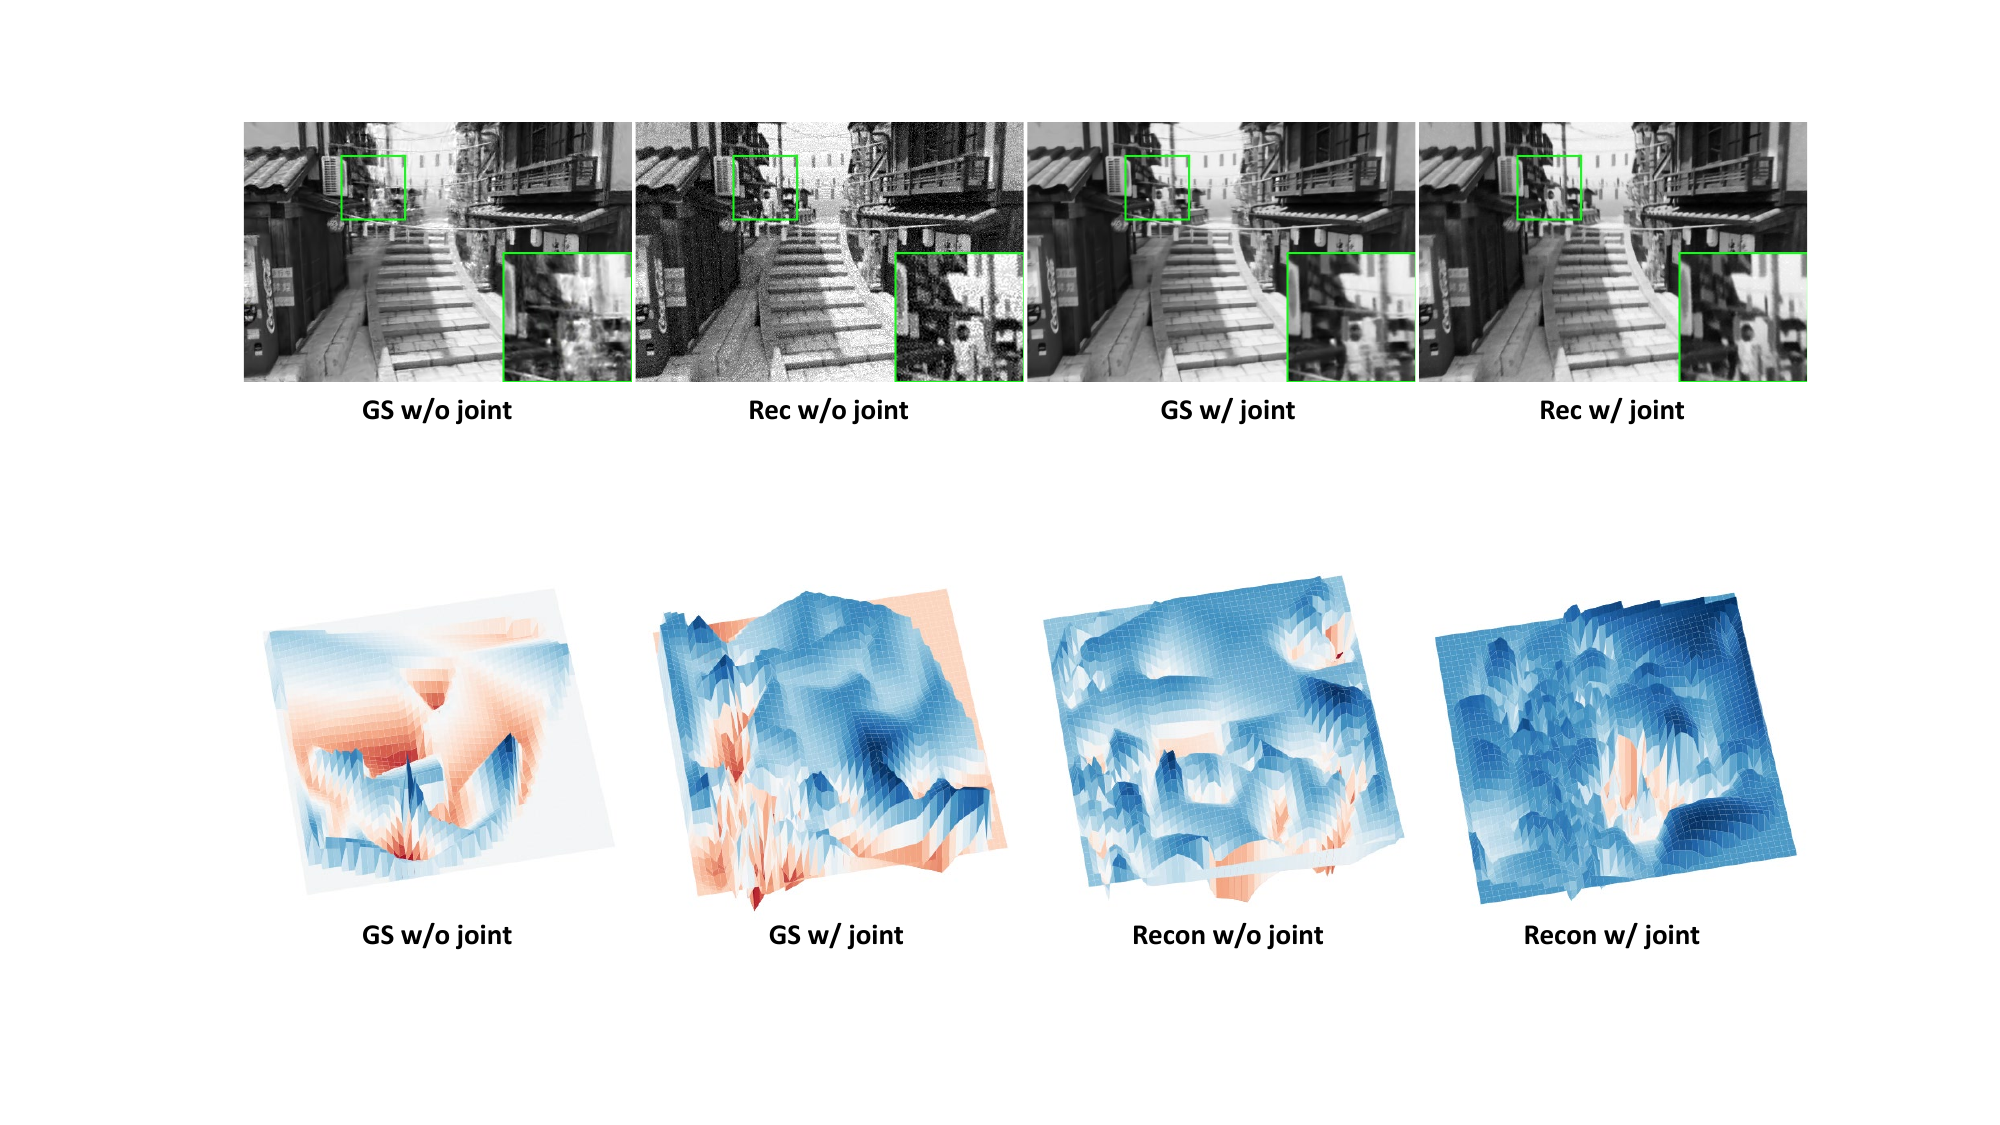}
    \caption{Image reconstruction visual ablation comparison of 3DGS and Recon-Net (with and without the joint optimization strategy).}
    \label{fig:sup:ablation}
\end{figure}
\subsection{Theorem: Effectiveness of the Joint Optimization Strategy}
\textbf{Theorem.}  
\textit{With our proposed collaborative optimization strategy, Spike-to-Image and 3D reconstruction tasks can mutually facilitate and enhance the optimization of each other.}
\\
\\
\noindent \textit{Proof.} Let the 3DGS output be $\mathbf{I}_{\text{gs}}$ and the Recon-Net output be $\mathbf{I}_{\text{rec}}$. Consider the scenario where 3DGS and Recon-Net are optimized independently, \ie, supervised by their respective loss functions. When training converges, the following conditions hold:
\begin{equation}
\left\{
\begin{aligned}
&\frac{\partial \mathcal{L}_{\text{gs}}}{\partial \mathbb{G}} = 0, \\
&\frac{\partial \mathcal{L}_{\text{gs}}}{\partial \mathbb{P}} = 0, \\
&\frac{\partial \mathcal{L}_{\text{rec}}}{\partial \theta} = 0.
\end{aligned}
\right.
\label{equ:sup:steady-equation}
\end{equation}

Building on the steady state of the optimization, \cref{fig:sup:ablation} provides a visual comparison of 3DGS and Recon-Net under their respective optimization. The figure shows that outputs from 3DGS and Recon-Net exhibit distinct characteristics in texture details and noise levels. Specifically, 3DGS outputs display reduced texture detail but achieve restoration with minimal noise. In contrast, Recon-Net produces sharper textures but is accompanied by substantial noise artifacts.

We model the outputs of 3DGS and Recon-Net with the image degradation model, formulated as follows:
\begin{equation}
\left\{
\begin{aligned}
    &\mathbf{I}_{\text{gs}} = A_{\text{gs}} \mathbf{I}_{\text{gt}} + n_{\text{gs}}, \\
    &\mathbf{I}_{\text{rec}} = A_{\text{rec}} \mathbf{I}_{\text{gt}} + n_{\text{rec}},
\end{aligned}
\right.
\end{equation}
where $\mathbf{I}_{\text{gt}}$ denotes the corresponding ground truth image, $A$ represents the degradation matrix and $n$ denotes the noise. Based on our observations in \cref{fig:sup:ablation}, the relationship between the degradation matrix and noise intensity for 3DGS and Recon-Net can be expressed as:
\begin{equation}
\| A_{\text{gs}} - \mathbf{I} \|^2 > \| A_{\text{rec}} - \mathbf{I} \|^2, \quad 
\| n_{\text{gs}} \|^2 < \| n_{\text{rec}} \|^2,    
\end{equation}
which indicates that 3DGS preserves structural details with less noise, while Recon-Net recovers sharper textures at the cost of higher noise intensity.

\begin{figure}
    \centering
    \includegraphics[width=0.8\linewidth]{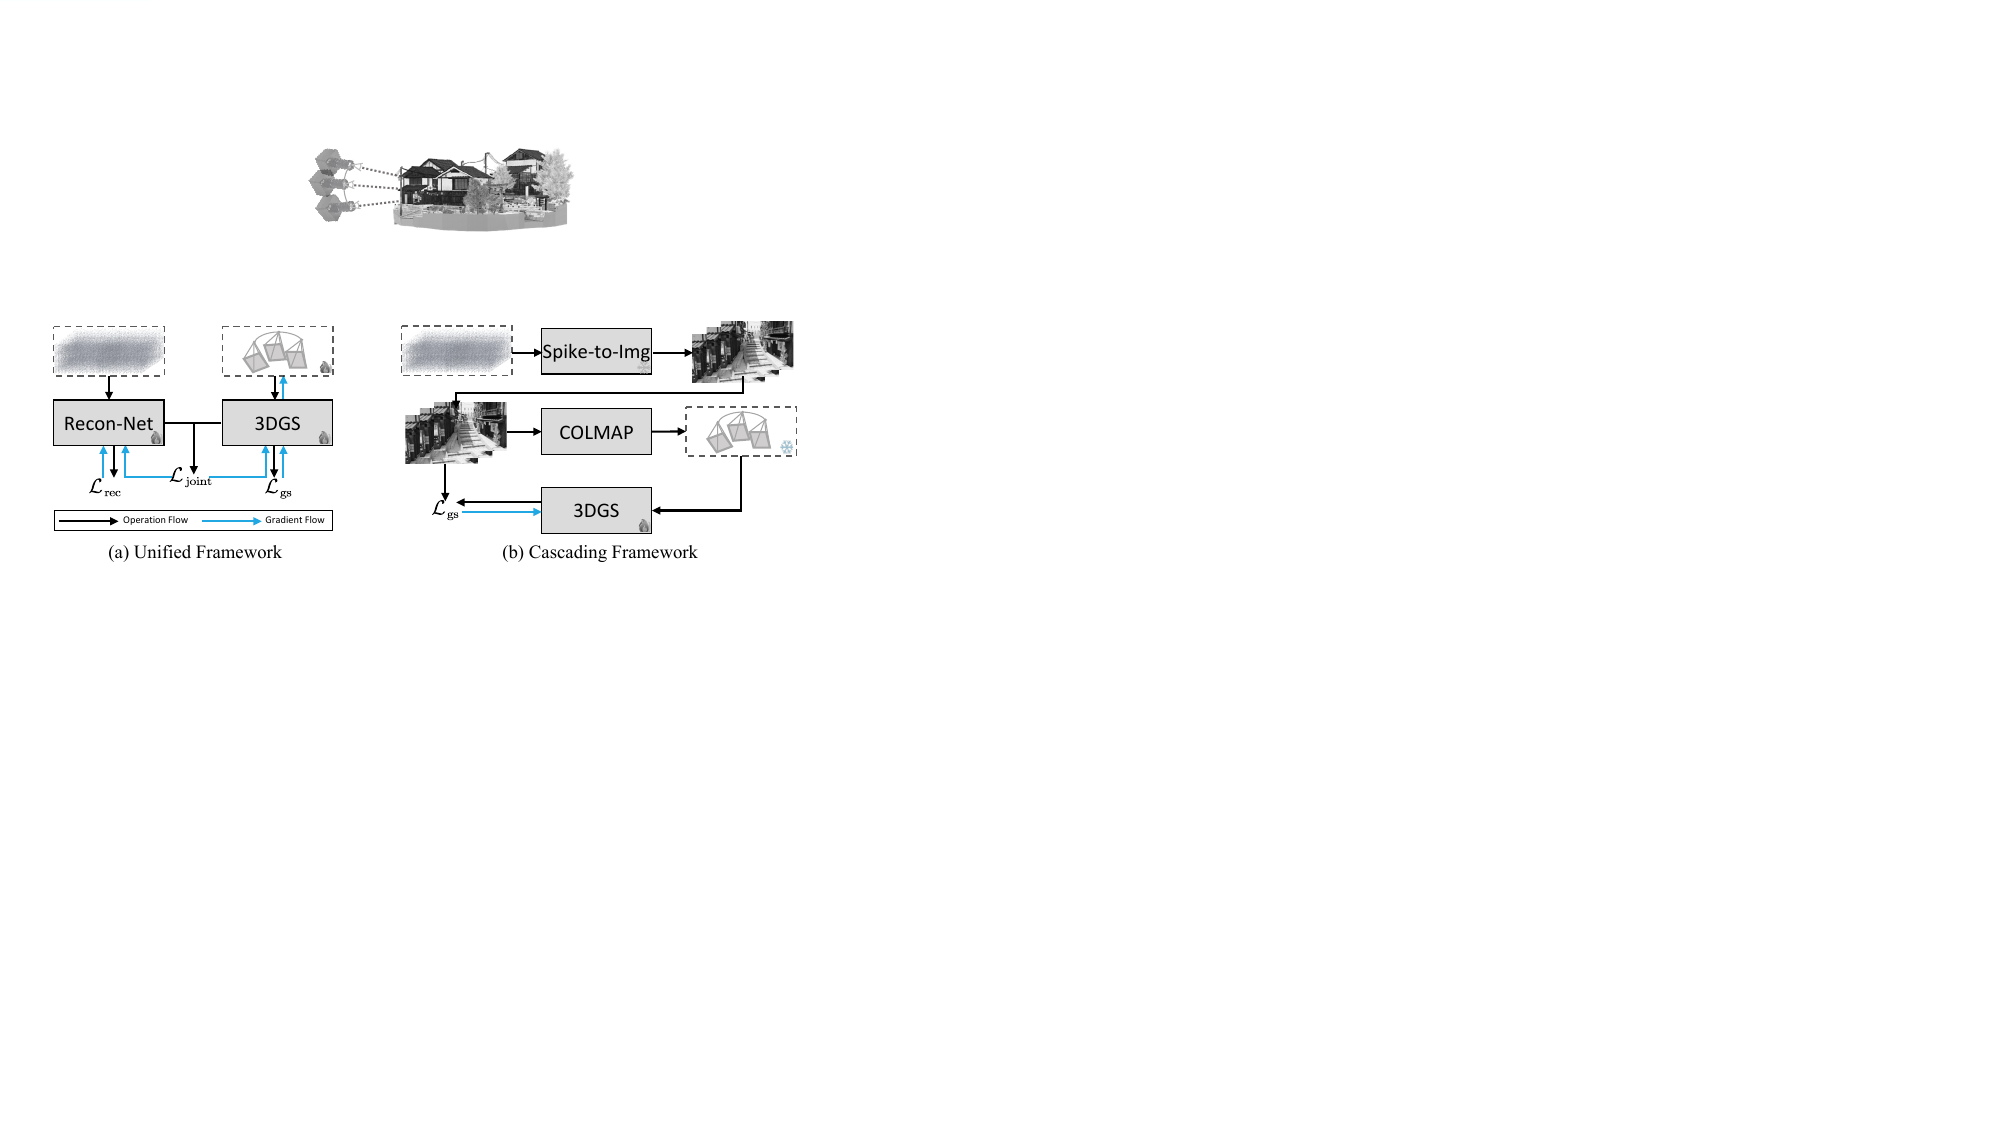}
    \caption{Framework comparison between our proposed unified optimization framework and previous cascading processing framework.}
    \label{fig:sup:comparison}
\end{figure}

In the following, we aim to analyze the contribution of the joint optimization loss on the equilibrium state of 3DGS and Recon-Net, with the \cref{equ:sup:steady-equation} re-formulated as:
\begin{equation}
\left\{
\begin{aligned}
&\frac{\partial \mathcal{L}_{\text{gs}}}{\partial \mathbb{G}} + \textcolor{red}{\frac{\partial \mathcal{L}_{\text{joint}}}{\partial \mathbb{G}}} = 0, \\
&\frac{\partial \mathcal{L}_{\text{gs}}}{\partial \mathbb{P}} + 
\textcolor{red}{\frac{\partial \mathcal{L}_{\text{joint}}}{\partial \mathbb{P}}} = 0, \\
&\frac{\partial \mathcal{L}_{\text{rec}}}{\partial \theta} + \textcolor{red}{\frac{\partial \mathcal{L}_{\text{joint}}}{\partial \theta}} = 0.
\end{aligned}
\right.
\end{equation}

Minimizing the expectation of the final loss function across different views $v$, we can obtain the optimal parameters for 3DGS, pose, and Recon-Net, with the optimization objective defined as follows:
\begin{align}
    \mathbb{P}^{*},\mathbb{G}^{*},\theta^{*} &= \arg\min_{\mathbb{P},\mathbb{G},\theta}\mathbb{E}_{v}  \big[ \mathcal{L}_{\text{gs}} + \mathcal{L}_{\text{rec}} +  \| \mathbf{I}_{\text{gs}} - \mathbf{I}_{\text{rec}} \|^2 \big] \label{sub:equ:1} \\
    &= \arg\min_{\mathbb{P},\mathbb{G},\theta}\mathbb{E}_{v}  \big[ \mathcal{L}_{\text{gs}} + \mathcal{L}_{\text{rec}} + \| A_{\text{gs}} \mathbf{I}_{\text{gt}} - A_{\text{rec}} \mathbf{I}_{\text{gt}} + n_{\text{gs}} - n_{\text{rec}} \|^2 \big] \label{sub:equ:2} \\
    &= \arg\min_{\mathbb{P},\mathbb{G},\theta}\mathbb{E}_{v}  \big[ \mathcal{L}_{\text{gs}} + \mathcal{L}_{\text{rec}} + \| A_{\text{gs}} - A_{\text{rec}} \|^2 \mathbf{I}_{\text{gt}}^2 + 
    2 (n_{\text{gs}} - n_{\text{rec}}) \odot  (A_{\text{gs}} - A_{\text{rec}}) \mathbf{I}_{\text{gt}} + \| n_{\text{gs}} - n_{\text{rec}} \|^2 \big] \label{sub:equ:3} \\
    &= \arg\min_{\mathbb{P},\mathbb{G},\theta}\mathbb{E}_{v}  \big[ \mathcal{L}_{\text{gs}} + \mathcal{L}_{\text{rec}} + \| A_{\text{gs}} - A_{\text{rec}} \|^2 \mathbf{I}_{\text{gt}}^2 + \| n_{\text{gs}} - n_{\text{rec}} \|^2 \big] \label{sub:equ:4} \\
    &= \arg\min_{\mathbb{P},\mathbb{G},\theta}\mathbb{E}_{v} \big[ \mathcal{L}_{\text{gs}} + \mathcal{L}_{\text{rec}} + \| A_{\text{gs}} - A_{\text{rec}} \|^2 \mathbf{I}_{\text{gt}}^2 +  n_{\text{rec}}^2 \big] \label{sub:equ:5}.
\end{align}
The transition from \cref{sub:equ:1} to \cref{sub:equ:2} involves substituting the degradation model into the optimization objective. 
Moving from \cref{sub:equ:2} to \cref{sub:equ:3}, the squared terms are expanded. 
From \cref{sub:equ:3} to \cref{sub:equ:4}, the cross-term is ignored due to the zero-mean property of the noise.
Finally, the step from \cref{sub:equ:4} to \cref{sub:equ:5} assumes that the noise intensity $n_{\text{gs}}$ is negligible, and the cross-term is omitted due to its zero-mean distribution.

For 3DGS, we extract the optimization objective for updating the Gaussian parameters and poses as:
\begin{equation}
   \mathbb{P}^{*},\mathbb{G}^{*} = \arg\min_{\mathbb{P},\mathbb{G}} \mathbb{E}_{v} \big[ \mathcal{L}_{\text{gs}} + \| A_{\text{gs}} - A_{\text{rec}} \|^2 \mathbf{I}_{\text{gt}}^2 \big].
\end{equation}
This optimization objective aligns the degradation matrix of 3DGS with that of Recon-Net. Since $A_{\text{rec}}$ typically exhibits weaker degradation, the alignment enhances the texture recovery capability of 3DGS.

For Recon-Net, the optimization target related to the network parameters $\theta$ is:
\begin{equation}
    \theta^* = \arg\min_{\theta} \mathbb{E}_{v}  \big[ \mathcal{L}_{\text{rec}} + \| A_{\text{gs}} - A_{\text{rec}} \|^2 \mathbf{I}_{\text{gt}}^2 + n_{\text{rec}}^2 \big].
\end{equation}
This objective aligns the degradation matrices of 3DGS and Recon-Net while minimizing the noise intensity of the Recon-Net outputs. Although this may slightly degrade $A_{\text{rec}}$, the resulting noise reduction significantly enhances overall performance.

To sum up, the joint optimization of 3DGS and Recon-Net promotes complementary information exchange, as illustrated in \cref{fig:sup:ablation}. Specifically, the collaborative optimization enhances the texture details in the images reconstructed by 3DGS and suppresses noise in the images recovered by Recon-Net.

\begin{figure}
    \centering
    \includegraphics[width=0.5\linewidth]{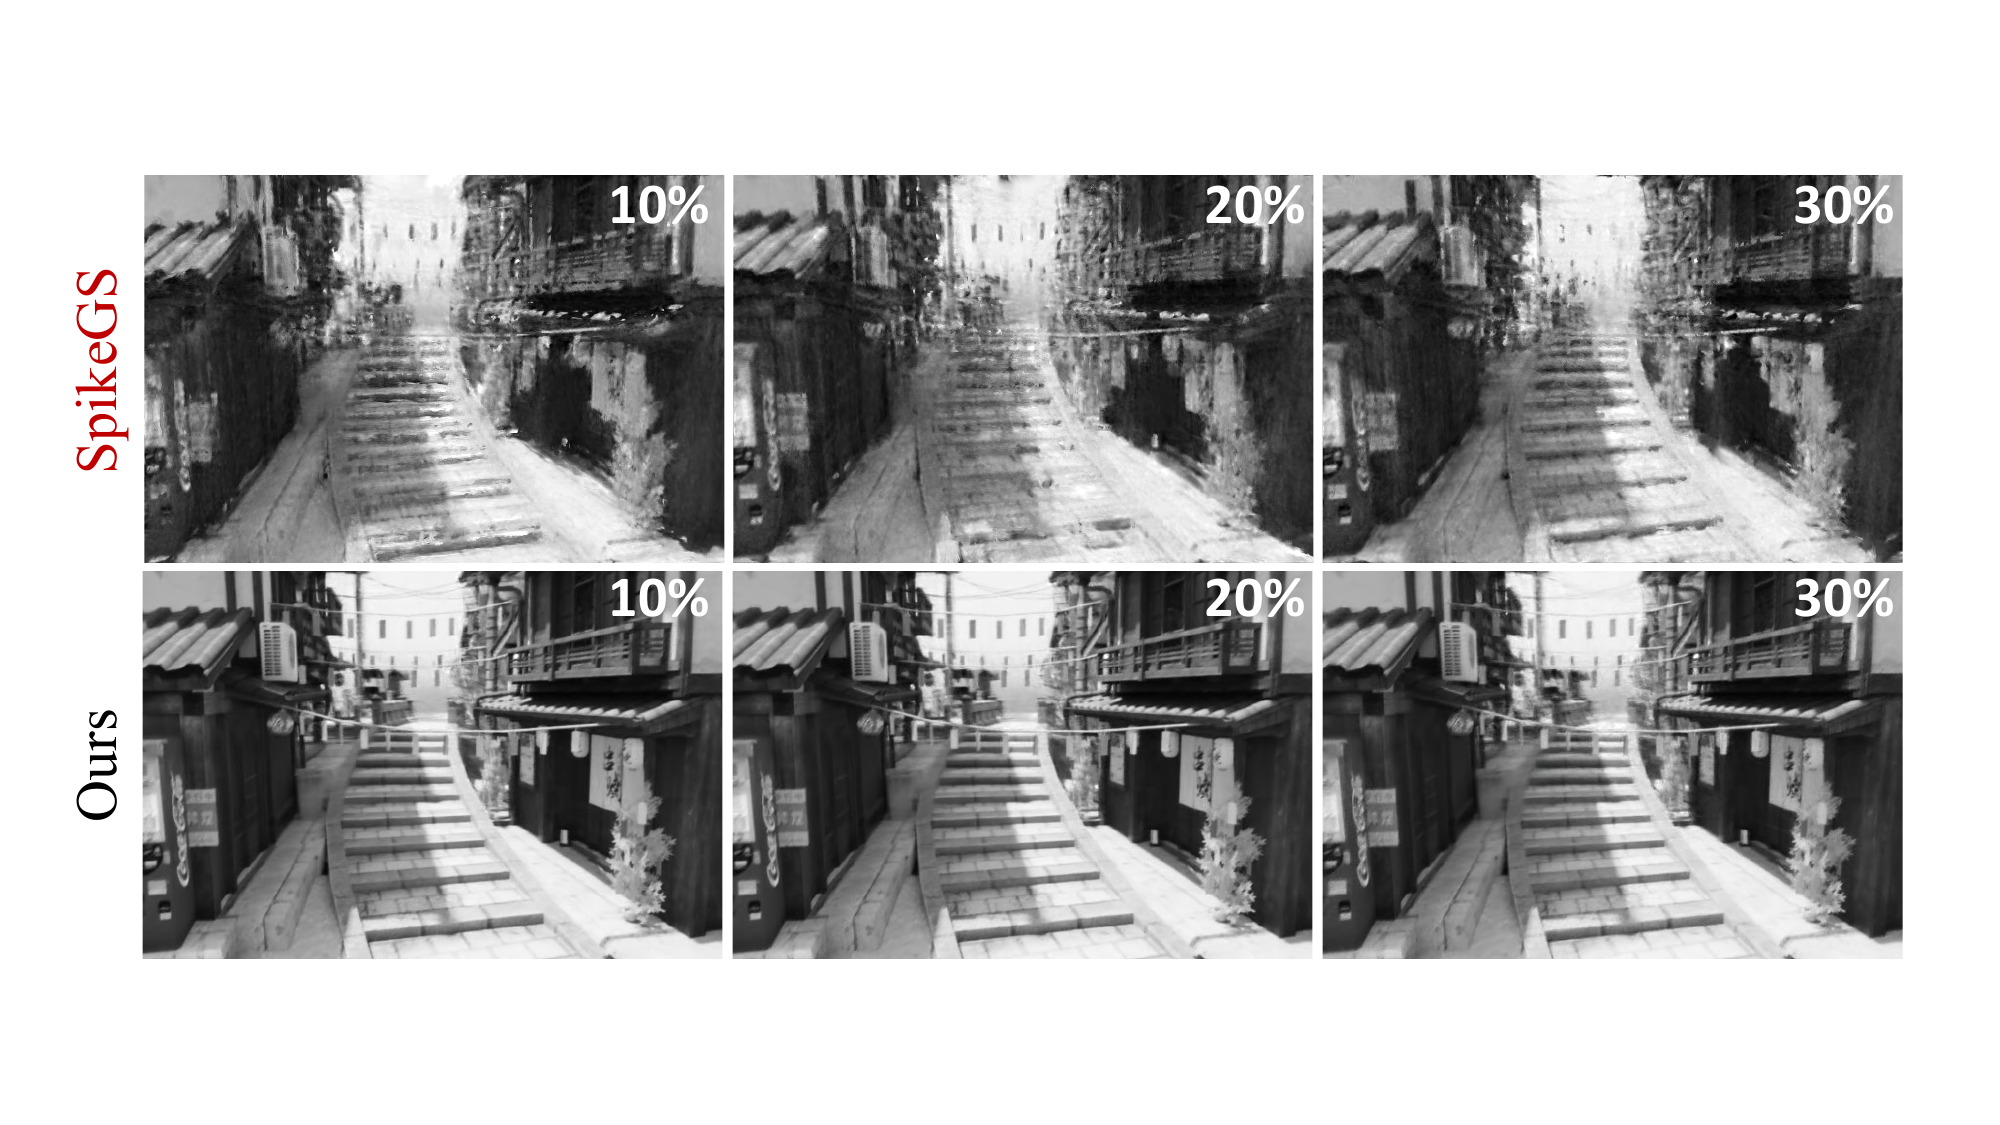}
    \caption{Visual comparison of our method with SpikeGS under inaccurate initial poses.}
    \label{fig:rgb_visual}
\end{figure}

\section{Framework Comparison} \label{sec:sup:framework}
We further elaborate on the main difference between our proposed unifid optimization framework and previous cascading frameworks, as illustrated in \cref{fig:sup:comparison}. Previous methods such as Spk2ImgNet-3DGS, and SpikeGS adopt the framework shown in \cref{fig:sup:comparison} (b), where a spike-to-image network is pre-trained to obtain high-quality image representations from the spike input. The subsequent processing follows the standard 3DGS pipeline, where the reconstructed image sequence is fed into COLMAP to estimate camera poses, which are further utilized to supervise the 3DGS training.

To address the potential issue of error propagation in cascading frameworks, we propose the joint optimization framework as shown in \cref{fig:sup:comparison} (a), which not only eliminates cascading errors but also leverages the complementary information provided by outputs of the 3DGS and Recon-Net to mutually enhance optimization, as demonstrated by our experiments and theoretical analysis.

\section{Implementation} \label{sec:sup:Implementation}
We extract 137 spike frames per viewpoint, with 97 frames employed to derive the long-exposure image specified in \cref{equ:3dgs_loss}. The remaining 20 frames at the beginning and end are designated for generating the short-exposure spike streams corresponding to the initial and final pose images. We set $M=13$, enabling each viewpoint to reconstruct a temporally uniform sequence of 13 frames. Our approach is implemented based on the BAD-Gaussian framework, with the Adam optimizer applied to optimize Recon-Net, pose estimations, and 3DGS parameters. All comparative analyses and ablation studies are performed on a single NVIDIA RTX 4090 GPU and an AMD EPYC 7742 64-Core Processor within the PyTorch framework. Besides, we employ the widely used metrics PSNR, SSIM, and LPIPS metrics to perform quantitative analysis.

\section{Network Architecture}  \label{sec:sup:network}
Our proposed Recon-Net employs a complementary long-short spike input format. The short-spike stream captures detailed motion features and rich textures, while the long-spike stream provides essential scene-level textural information, effectively reducing noise embedded in the short-spike stream.

The network architecture is illustrated in \cref{fig:framework}. 
Specifically, the short-spike input comprises 41 frames of binary 0-1 spikes, while the long-spike input is voxelized by partitioning 137 input spike frames into groups of four, aggregating each group (with intermediate frames omitted), resulting in 34 voxel frames. Features from the short-spike and voxelized long-spike inputs are extracted and channel-aligned through an initial pre-processing convolutional layer. These aligned features are subsequently fused with the time index via a summation operation, enabling the integration of temporal and spatial information. Finally, the fused representation is passed through a sequence of convolutional blocks to extract deeper features, culminating in the reconstruction of the output image.

\section{Experimental Details}  \label{sec:sup:exp}
We present further 3D reconstruction visual comparison results between our proposed method and previous methods on the synthetic dataset as shown in \cref{fig:sup:compare_1}, with the visual comparison on the inaccurate initial poses dataset depicted in \cref{fig:sup:ablation_model}. 

Additionally, we conduct quantitative and qualitative comparisons of USP-Gaussian and previous approaches on the spike-to-image task as shown in \cref{fig:sup:compare_1,tab:sup:tab1}. The spike-based image reconstruction methods for TFP-3DGS, TFI-3DGS, and Spk2ImgNet-3DGS correspond to TFI, TFI, and Spk2ImgNet respectively. SpikeNeRF reconstructs spike frames based on the accumulated spike input, while SpikeGS reconstructs initial images based on the BSN.

The quantitative performance comparison is described in \cref{tab:sup:tab1} and the visual comparison is depicted in \cref{fig:sup:compare_1}. Specifically, Long-TFP corresponds to reconstructing the image accumulated over 97 frames, and Short-TFP corresponds to those accumulated over 41 frames. From the visual comparison, it can be observed that supervised method Spk2ImgNet suffers from performance degradation due to the dataset domain gap and the self-supervised method in SpikeGS heavily relies on the BSN, which leads to significant artifacts when the input spike stream embodies a high signal-to-noise ratio and rich image details. 

In contrast, our proposed USP-Gaussian achieves joint optimization while simultaneously training the Recon-Net, thereby introducing a novel self-supervised spike-based image reconstruction framework. Leveraging the multi-view constraint provided by 3DGS, our method demonstrates superior self-supervised image reconstruction performance.

\begin{figure*}[t]
\centering
\begin{subfigure}{\textwidth}
\centering
\includegraphics[width=0.95\textwidth]{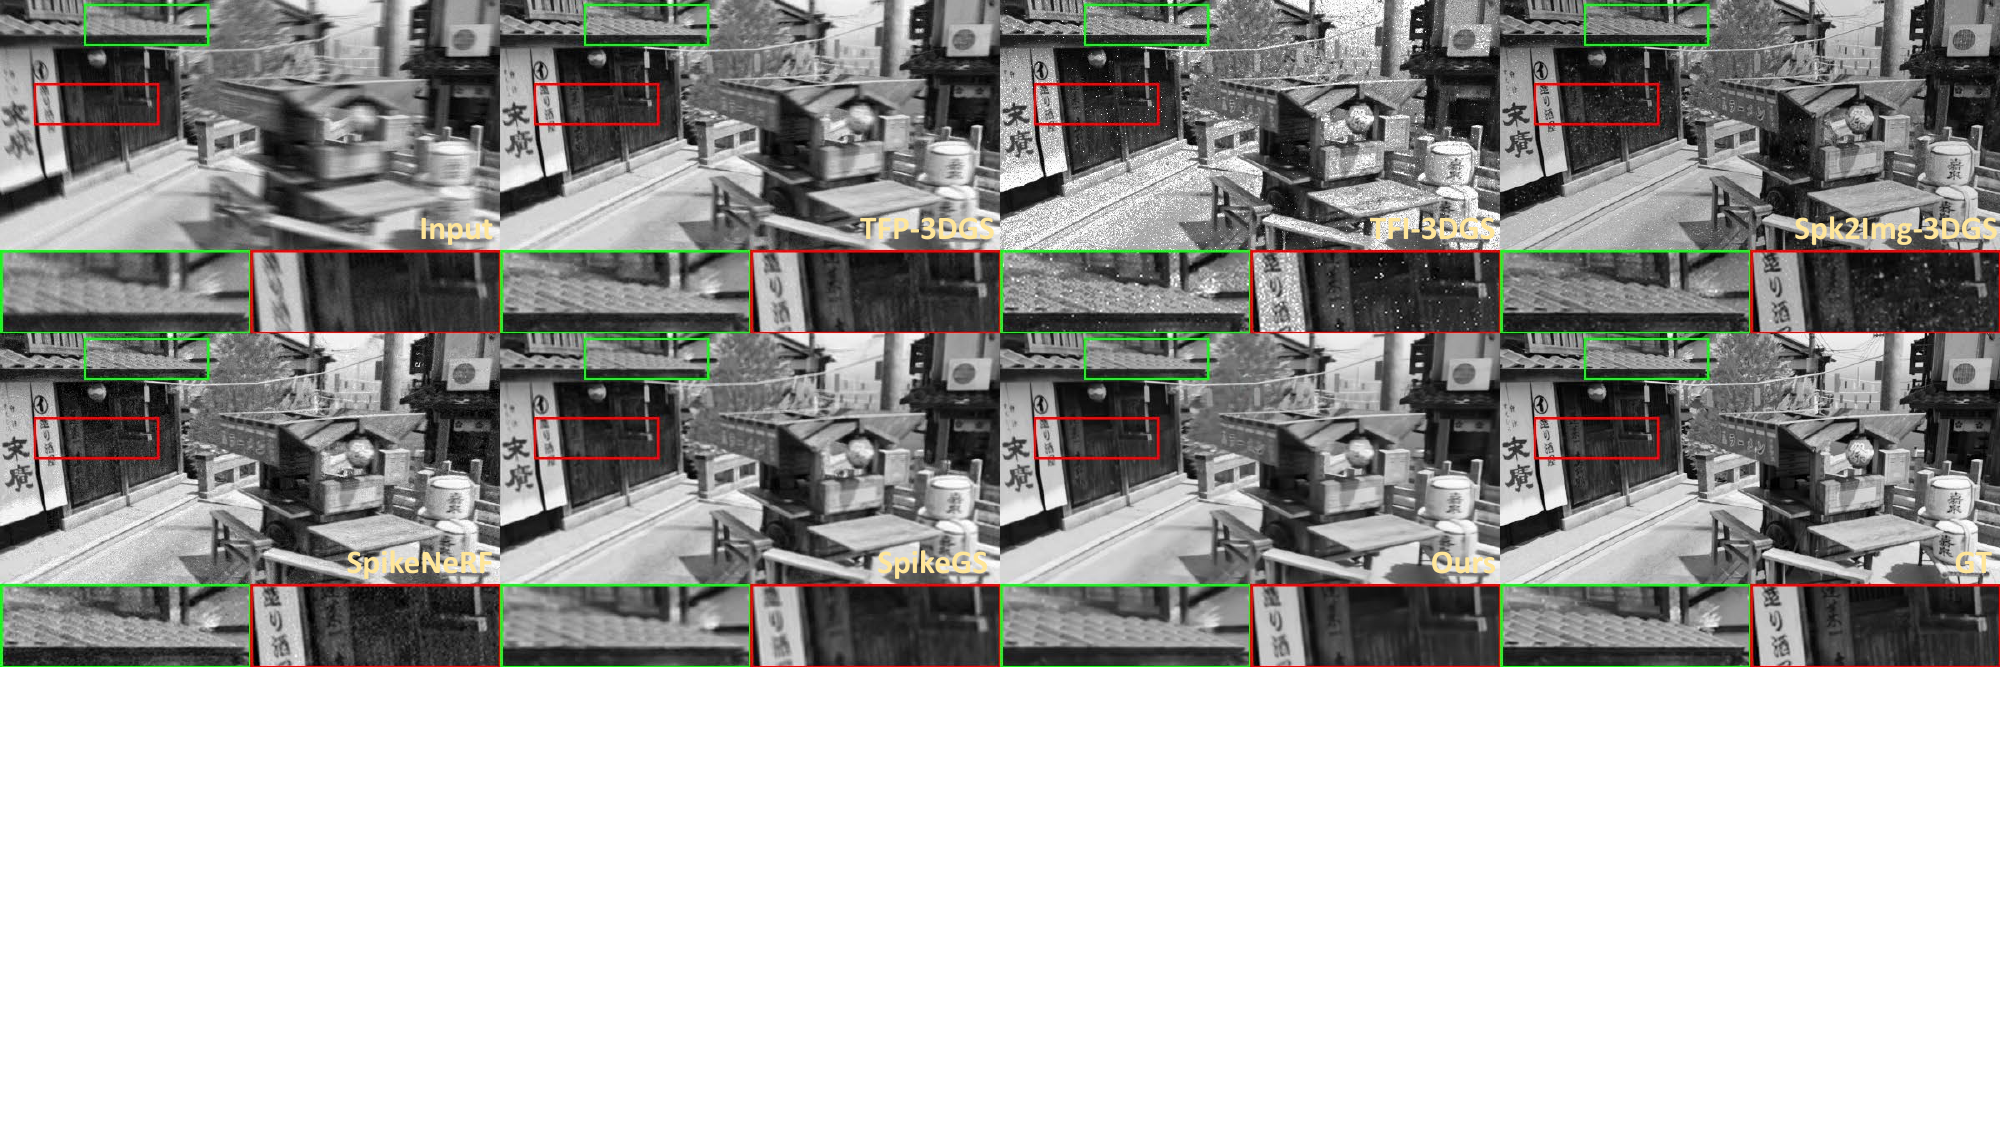}
\vspace{-0.05cm}
\end{subfigure} 
\begin{subfigure}{\textwidth}
\centering
\includegraphics[width=0.95\textwidth]{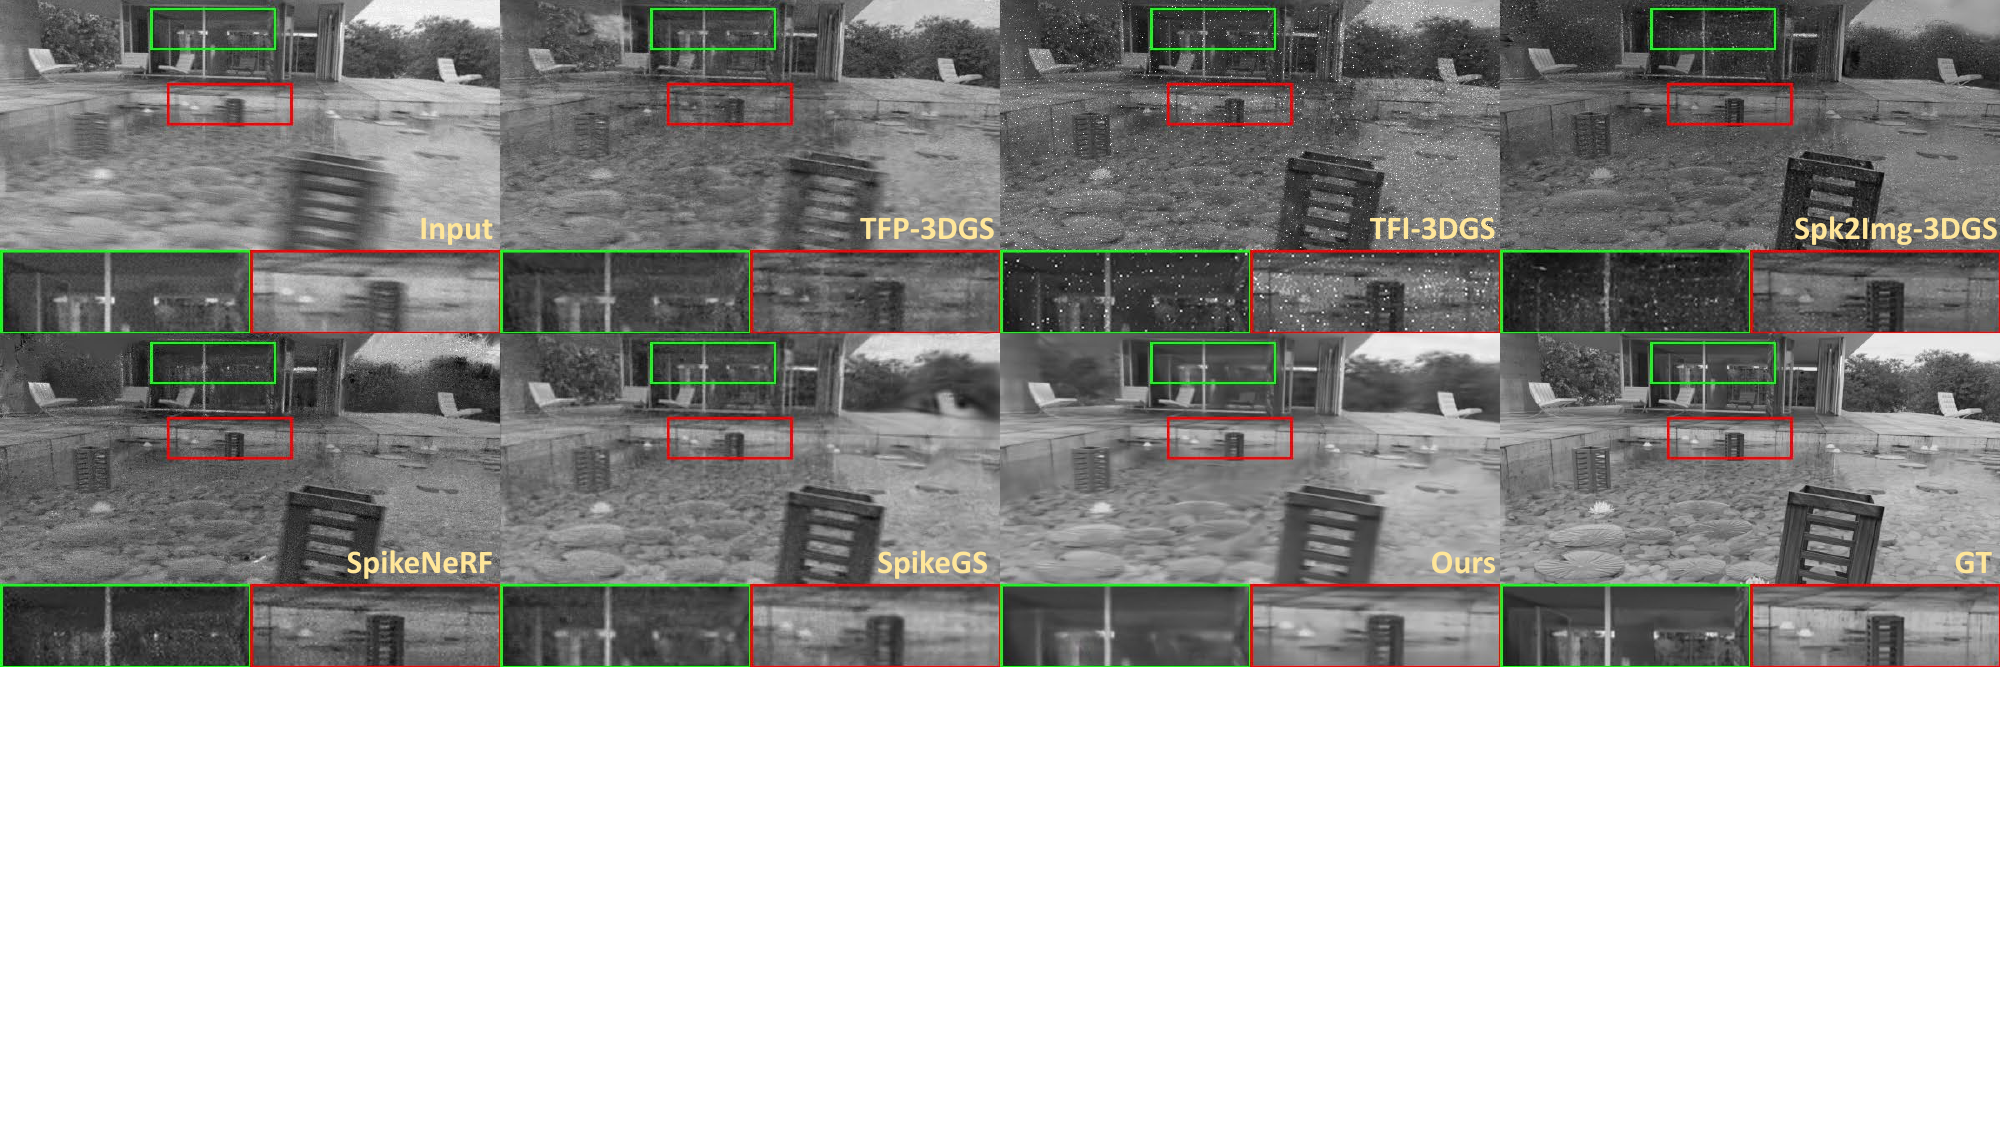}
\end{subfigure}
\caption{3D reconstruction visual comparison of our USP-Gaussian compared with previous methods on the synthetic dataset, where the input is the long-exposure image defined in \cref{equ:tfp}.}

\label{fig:sup:compare_1}
\end{figure*}

% \begin{figure}[t]
%     \centering
%     % First animation
%     \centering
%     \animategraphics[width=\linewidth, autoplay, loop]{3}{imgs_abl/abl_}{2}{31}
%     \caption{Video restoration of our optimized 3DGS and Recon-Net on the synthetic scene across different views, where Input denotes the long-exposure image formulated from the spike. It is recommended to view this gif using Acrobat PDF reader.}
%     \label{sup_fig:animations}
% \end{figure}
\begin{table*}[t]
\vspace{-1em}
\caption{Spike-to-Image reconstruction quantitative comparison on the synthetic dataset.}
\label{tab:sup:tab1}
\centering
\resizebox{\textwidth}{!}{ 
\begin{tabular}{lccc cccc cccc cccc cccc} 
\toprule[2pt]
\multirow{2}{*}{Methods} & \multicolumn{3}{c}{Wine} & & \multicolumn{3}{c}{Tanabata} & & \multicolumn{3}{c}{Factory} & & \multicolumn{3}{c}{Outdoor Pool} & & \multicolumn{3}{c}{Average} \\ 
\cmidrule(lr){2-4} \cmidrule(lr){6-8} \cmidrule(lr){10-12} \cmidrule(lr){14-16} \cmidrule(lr){18-20}
                    & PSNR & SSIM & LPIPS & & PSNR & SSIM & LPIPS & & PSNR & SSIM & LPIPS & & PSNR & SSIM & LPIPS & & PSNR & SSIM & LPIPS \\ 
\midrule
TFP        & 23.174 & 0.637 & 0.403 & & 23.951 & 0.630 & 0.444 & & 26.794 & 0.684 & 0.332 & & 28.101 & 0.633 & 0.495 & & 24.100 & 0.614 & 0.394 \\
TFI       & 20.368 & 0.537 & 0.563 & & 19.415 & 0.460 & 0.678 & & 22.067 & 0.561 & 0.530 & & 22.694 & 0.471 & 0.758 & & 20.001 & 0.484 & 0.594 \\
Spk2ImgNet   & 20.443 & 0.688 & 0.291 & & 19.853 & 0.653 & 0.364 & & 22.905 & 0.651 & 0.376 & & 23.566 & 0.504 & 0.652 & & 20.513 & 0.599 & 0.388 \\
SpikeNeRF  & 23.909 & 0.598 & 0.411 & & 24.242 & 0.562 & 0.473 & & 25.252 & 0.585 & 0.407 & & 25.478 & 0.477 & 0.615 & & 23.446 & 0.532 & 0.446 \\
SpikeGS    & \cellcolor{orange!25}24.981 & \cellcolor{orange!25}0.764 & \cellcolor{orange!25}0.263 & & \cellcolor{orange!25}25.810 & \cellcolor{orange!25}0.767 & \cellcolor{orange!25}0.290 & & \cellcolor{orange!25}28.298 & \cellcolor{orange!25}0.794 & \cellcolor{orange!25}0.192 & & \cellcolor{orange!25}29.443 & \cellcolor{orange!25}0.759 & \cellcolor{orange!25}0.323 & & \cellcolor{orange!25}25.661 & \cellcolor{orange!25}0.733 & \cellcolor{orange!25}0.251 \\
Ours          & \cellcolor{red!25}27.138 & \cellcolor{red!25}0.855 & \cellcolor{red!25}0.178 & & \cellcolor{red!25}27.539 & \cellcolor{red!25}0.834 & \cellcolor{red!25}0.222 & & \cellcolor{red!25}29.434 & \cellcolor{red!25}0.849 & \cellcolor{red!25}0.173 & & \cellcolor{red!25}31.154 & \cellcolor{red!25}0.833 & \cellcolor{red!25}0.255 & & \cellcolor{red!25}27.259 & \cellcolor{red!25}0.801 & \cellcolor{red!25}0.194 \\
\bottomrule[2pt]
\end{tabular}
}
\end{table*}

\begin{figure*}[t]
\centering
\begin{subfigure}{\textwidth}
\centering
\includegraphics[width=0.95\textwidth]{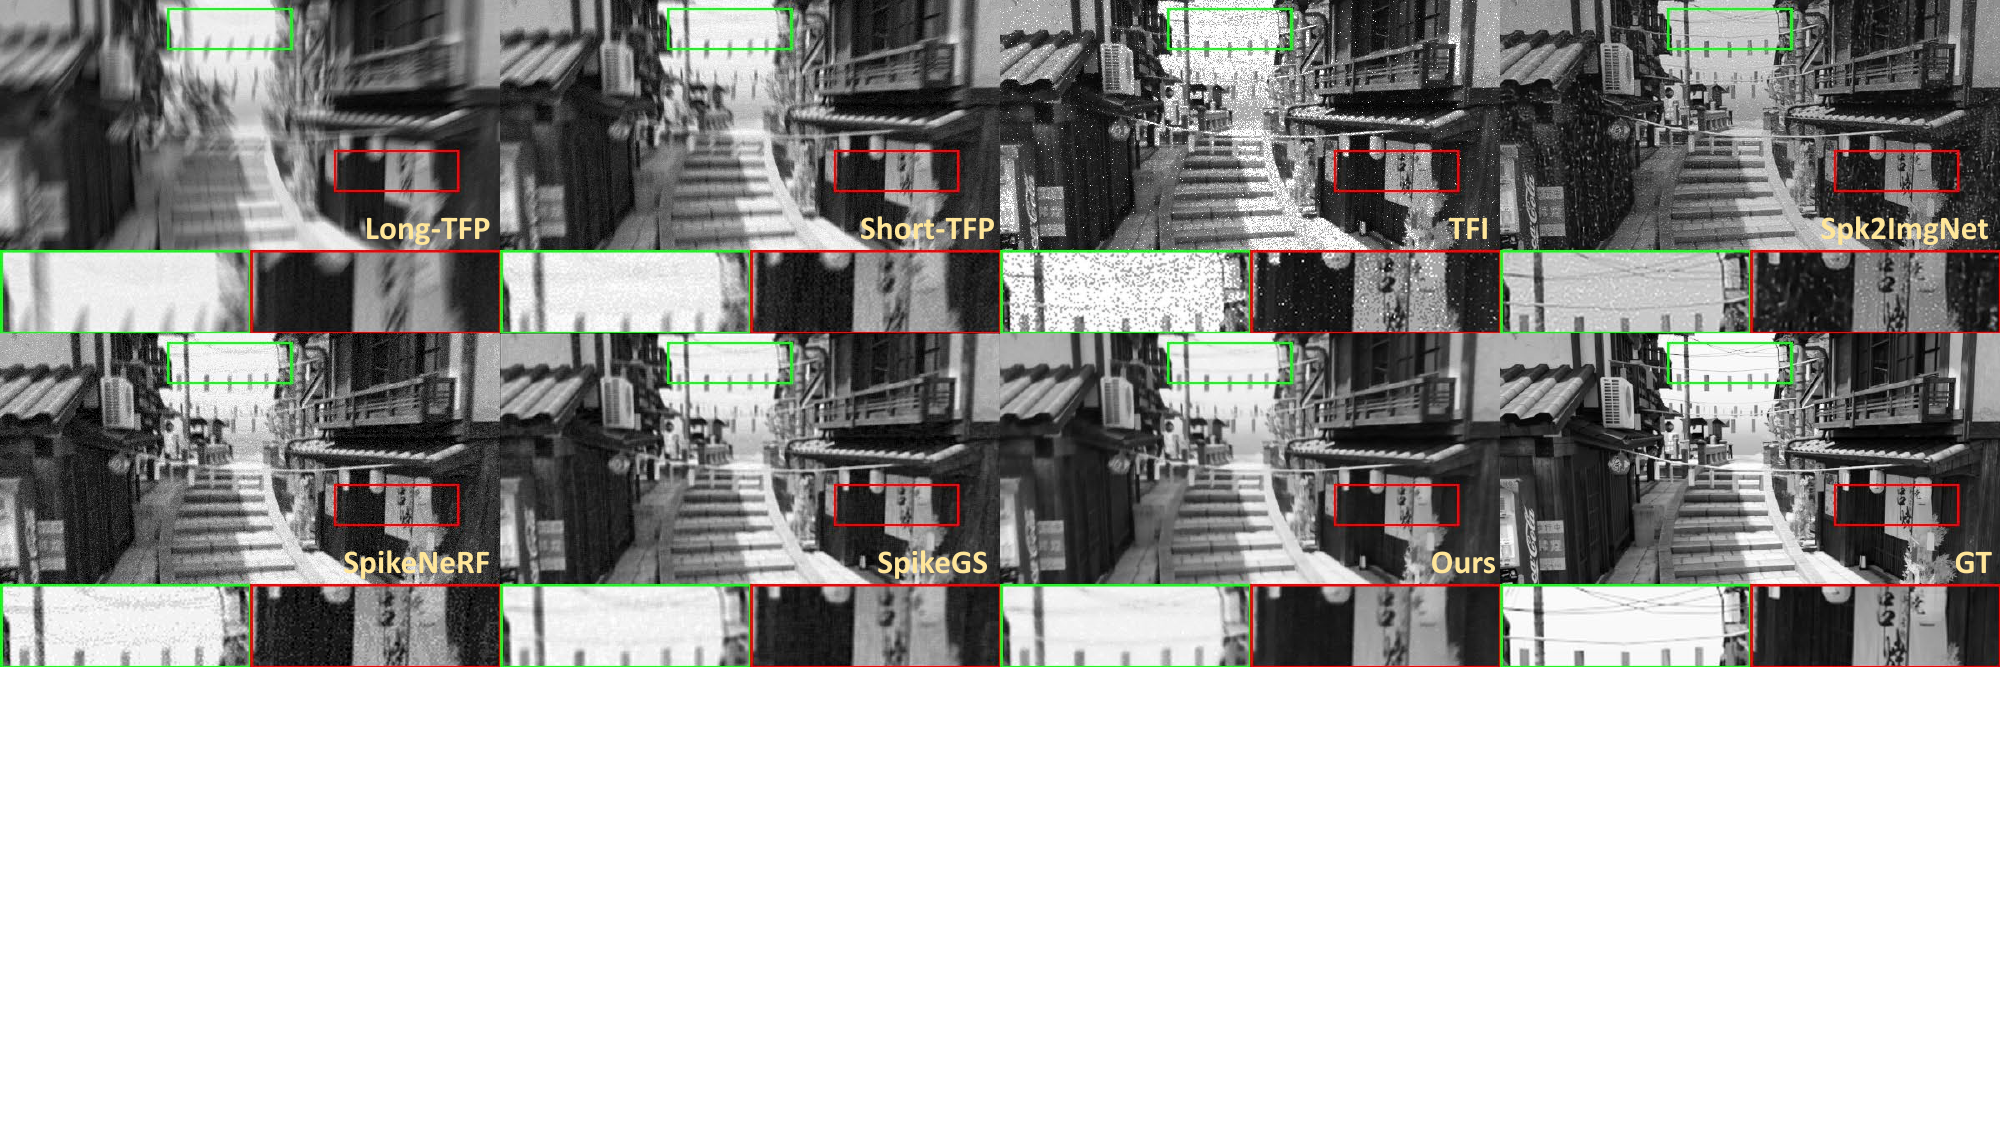}
\vspace{-0.05cm}
\end{subfigure} 
\begin{subfigure}{\textwidth}
\centering
\includegraphics[width=0.95\textwidth]{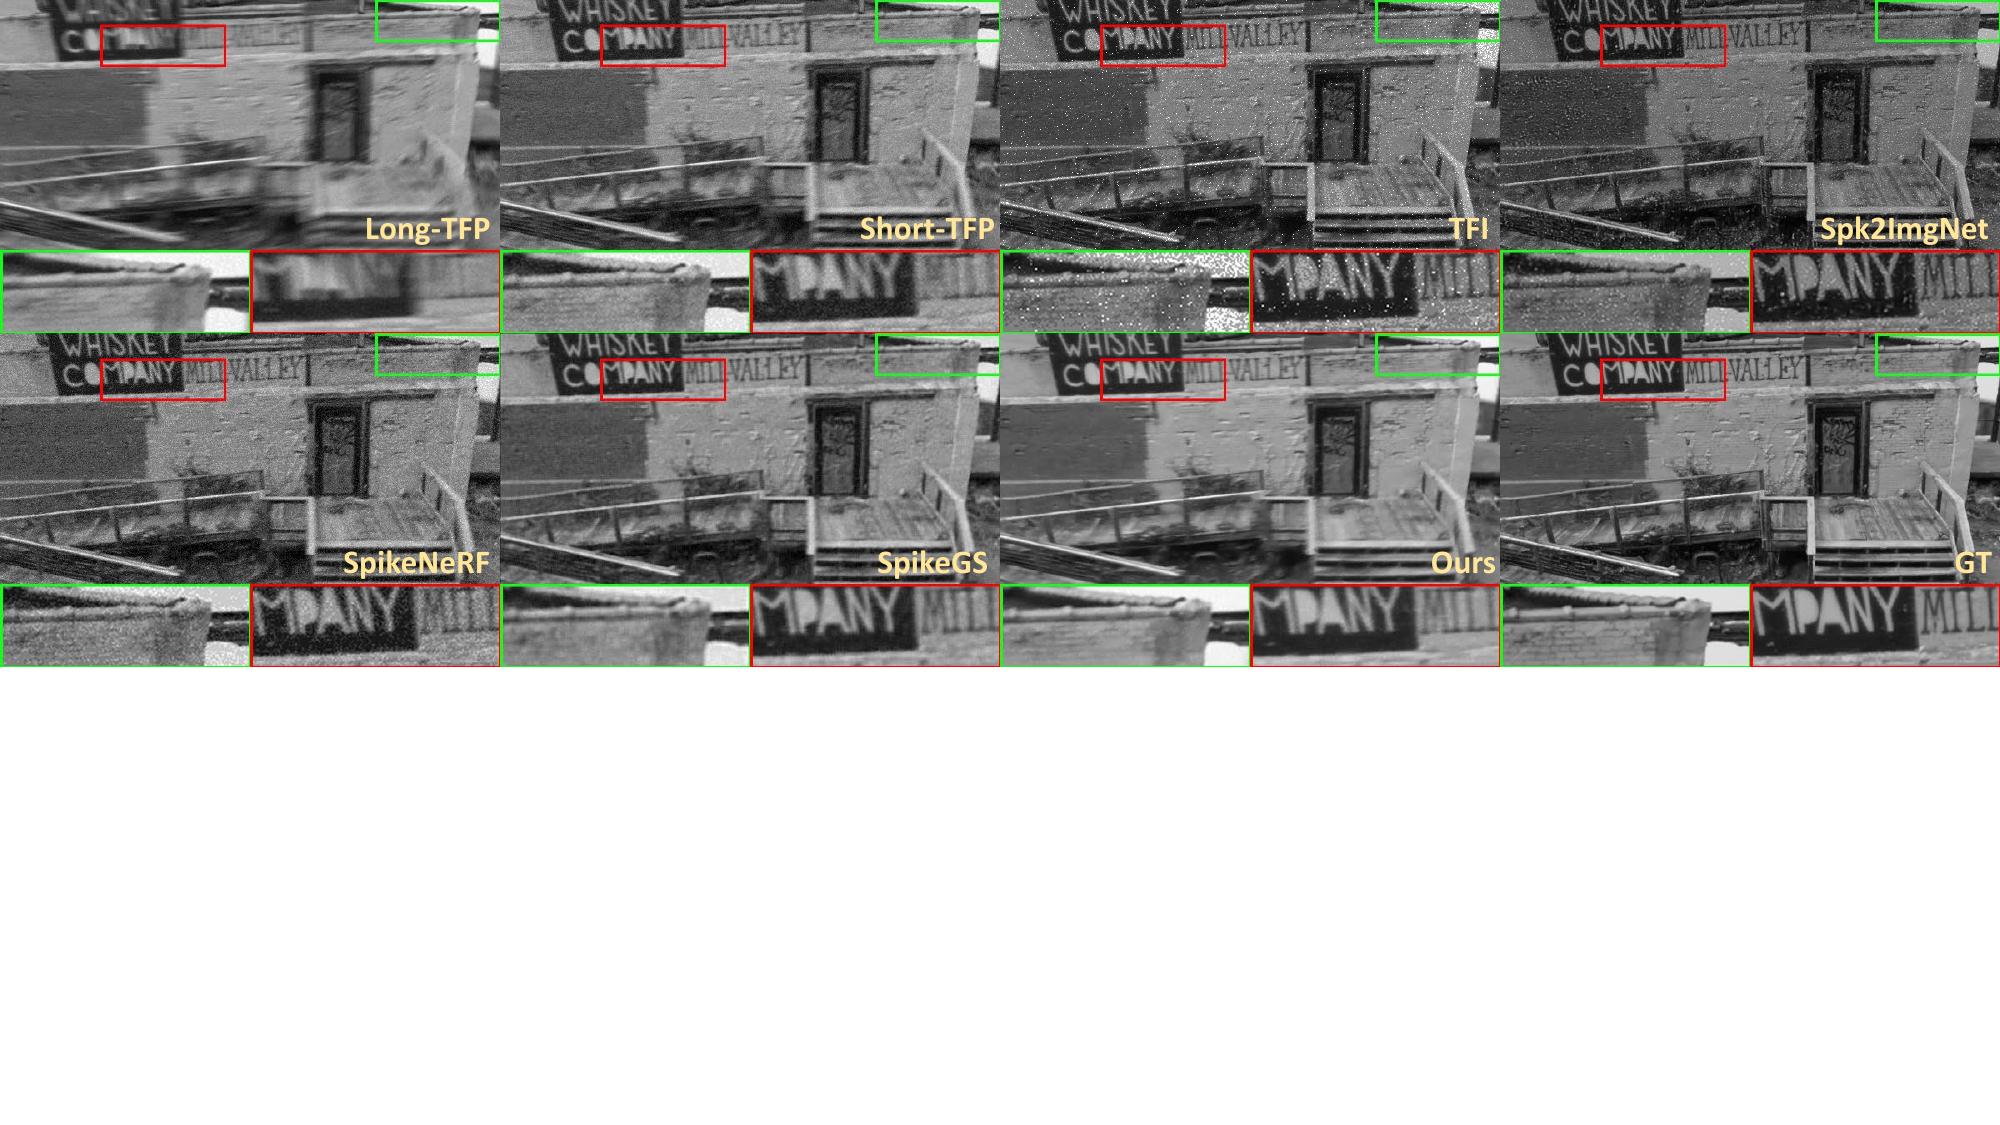}
\vspace{-0.05cm}
\end{subfigure}
\begin{subfigure}{\textwidth}
\centering
\includegraphics[width=0.95\textwidth]{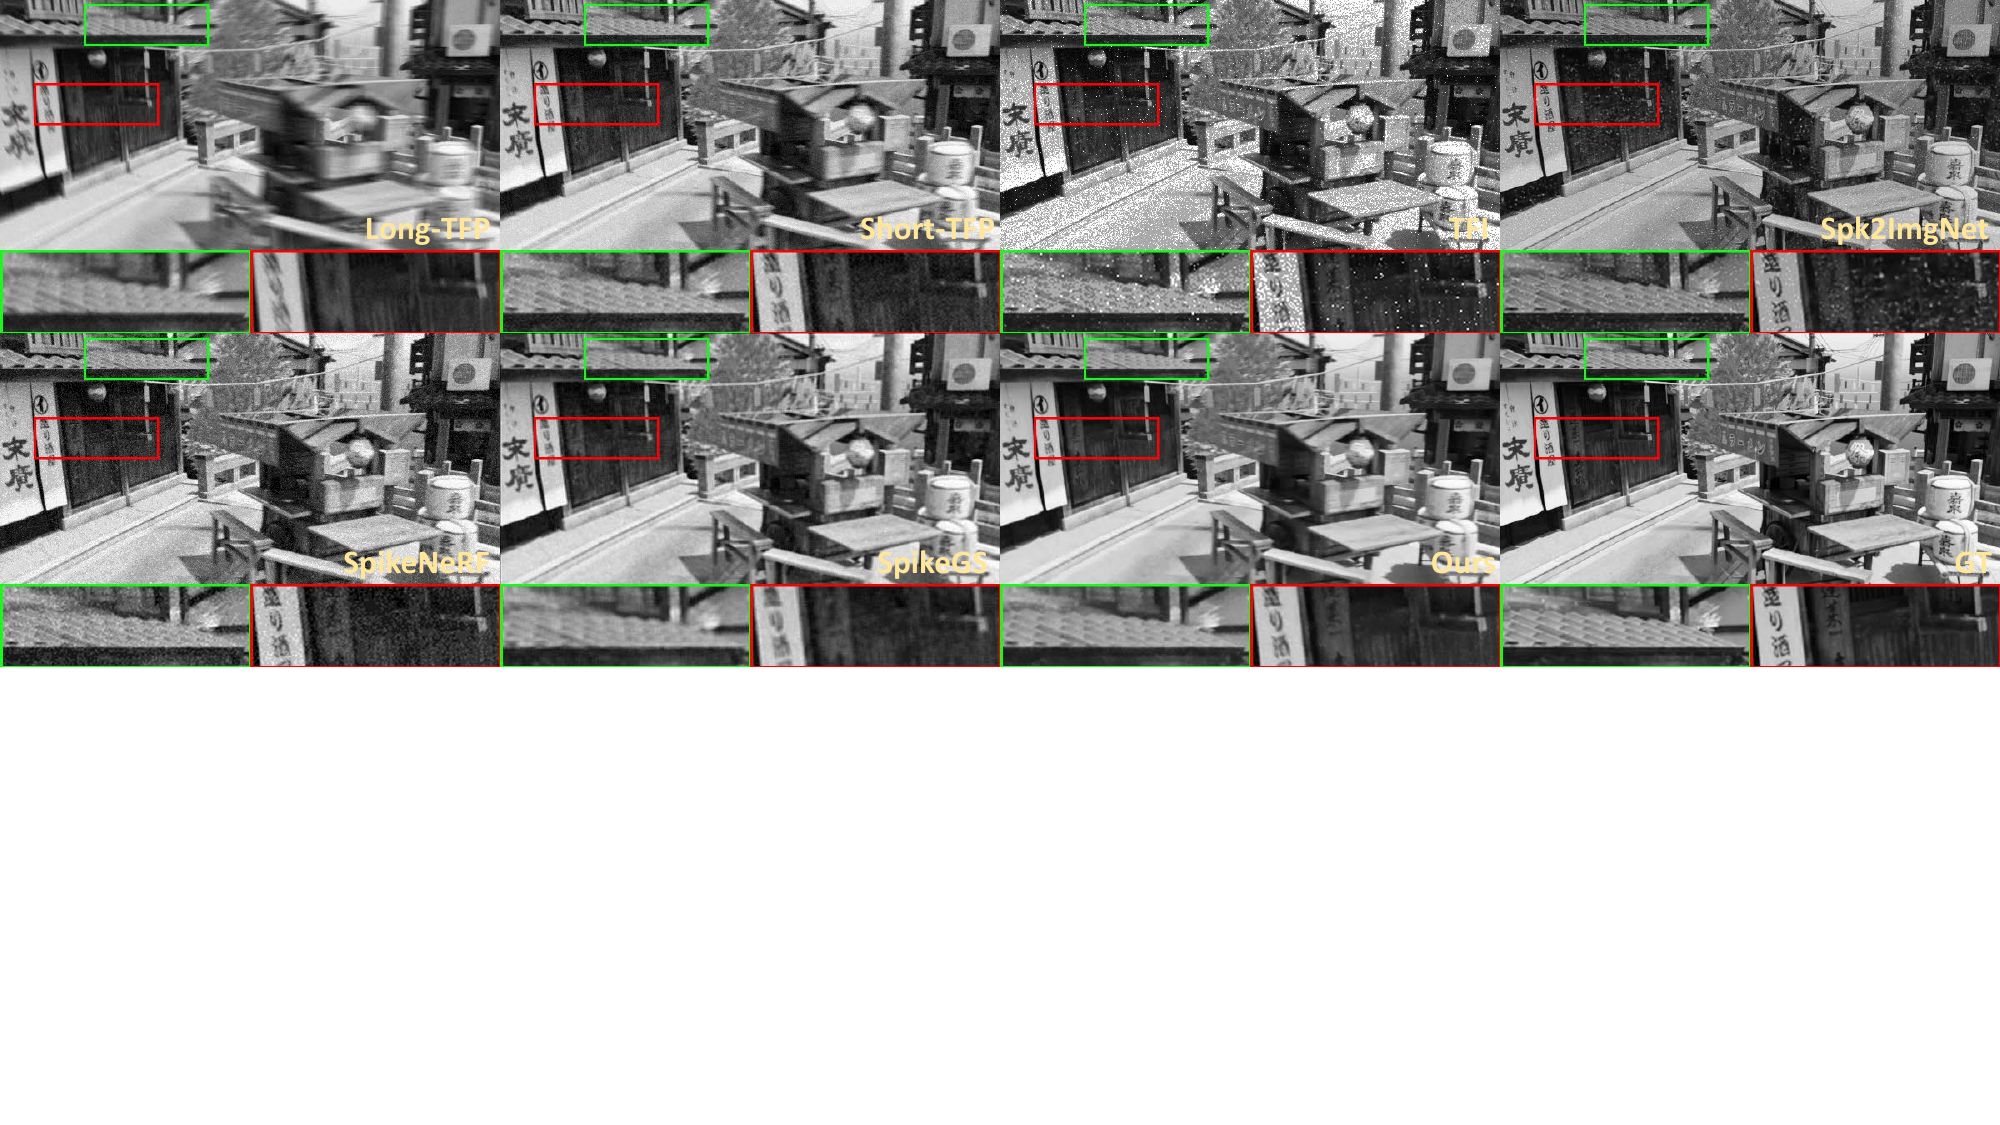}
\vspace{-0.05cm}
\end{subfigure} 
\begin{subfigure}{\textwidth}
\centering
\includegraphics[width=0.95\textwidth]{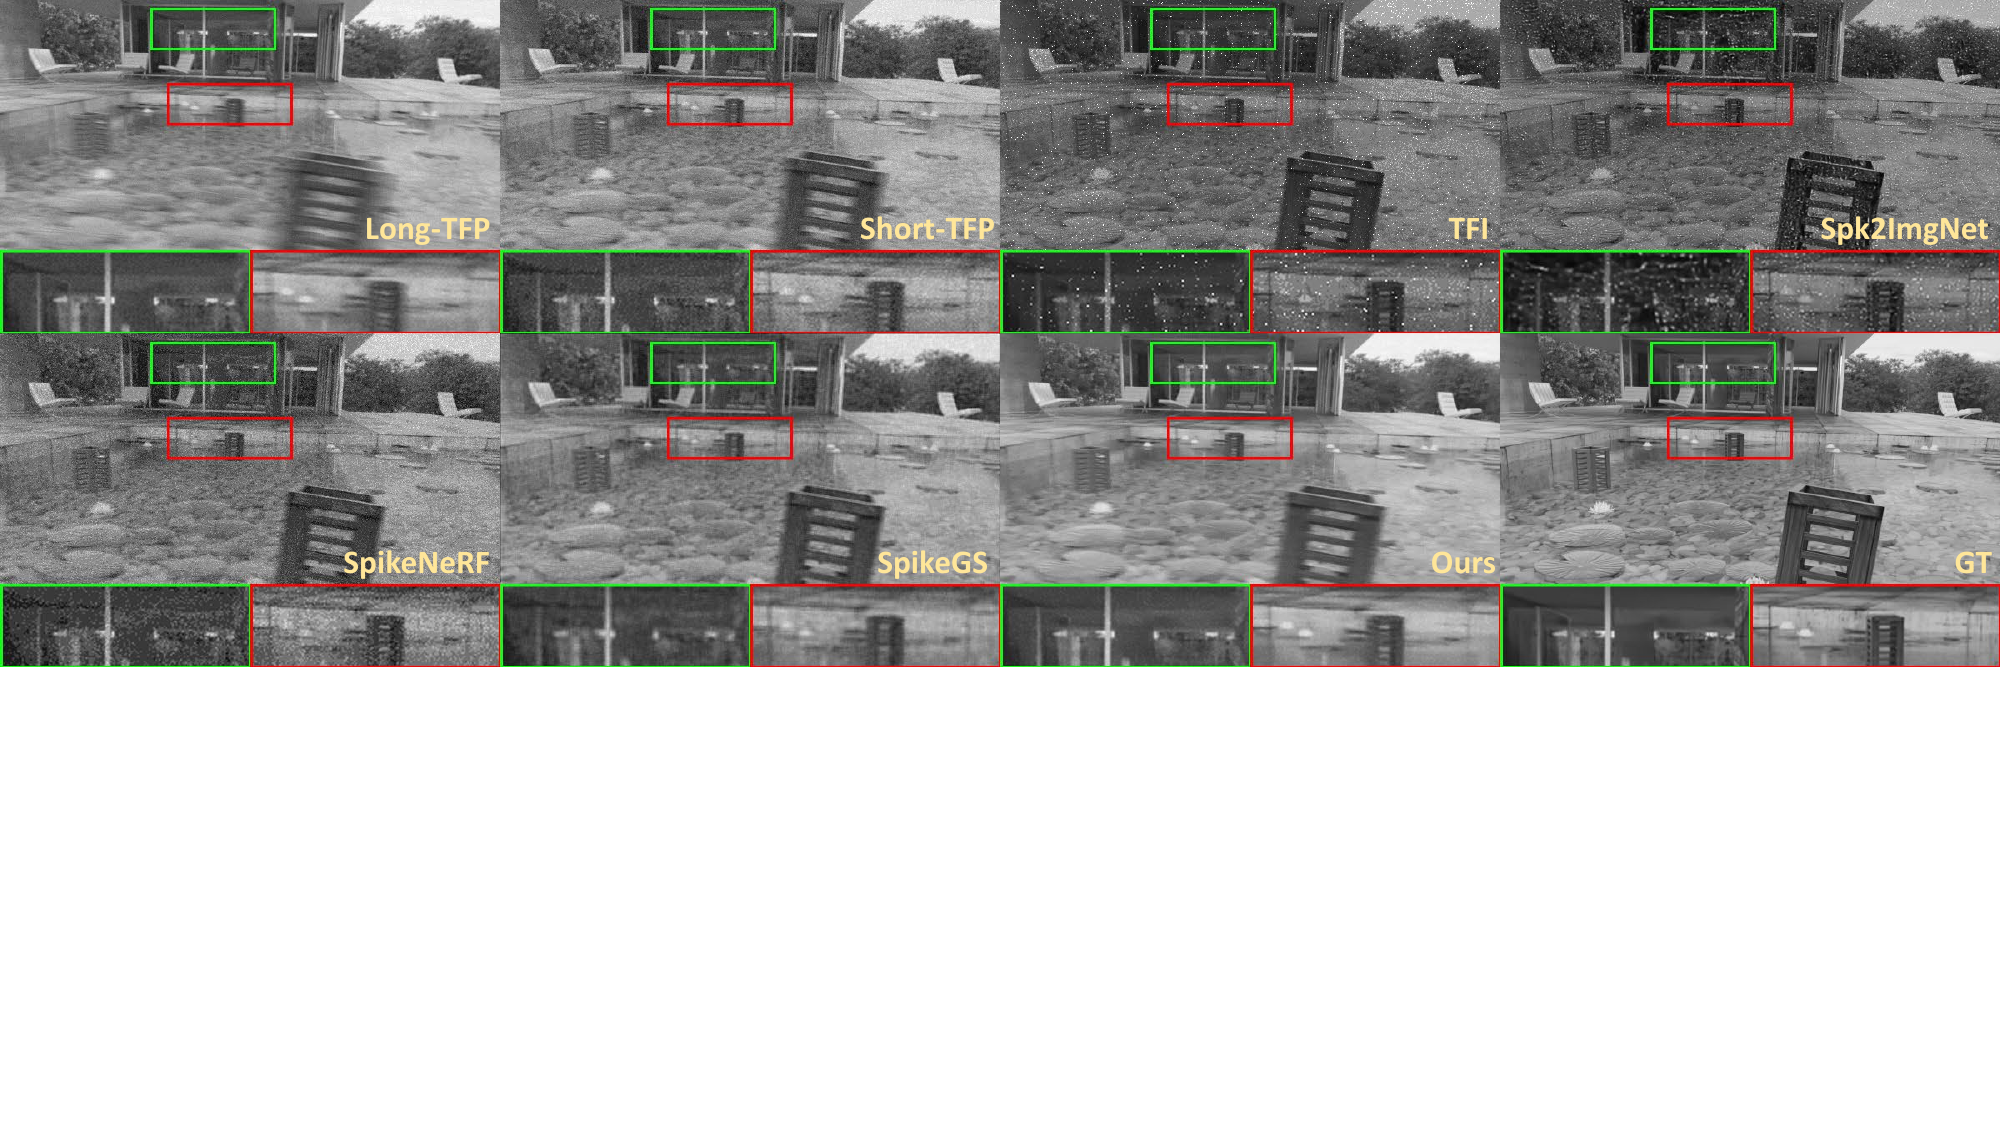}
\end{subfigure}
\caption{Spike-to-image reconstruction comparison of our USP-Gaussian compared with previous methods on the synthetic dataset.}
\end{figure*}

% {
%     \newpage
%     \small
%     \bibliographystyle{ieeenat_fullname}
%     \bibliography{main}
% }
